# Supplementary material for: Multi-Step Inference for Reasoning Over Paragraphs
Source: arXiv:2004.02995 source file (2021-06-07)
Supplement: Supplementary file 1 [file appendix.tex]

\section{Hyperparameters}
All the models share the same hyperparameters, which are shown in Table \ref{hyper}.
\section{Span encoder}
The reranker aims to choose the best candidates as the final answer. We represent each candidate as a vector by the end-point method. The candidate representation $x_{(i,j)}$ is the concatenation of the start token representations and the end token representations, i.e.~$x_{(i,j)} = [x_i ; x_j]$.

% \end{document}
